# Supplementary material for: Interface-induced Topological Insulator Transition in GaAs/Ge/GaAs Quantum Wells
Source: arXiv:1308.6353 source file (2013-08-29)
Supplement: Supplementary file 1 [file Supplemental_material.pdf]

# Supplemental Material for Interface Polarization Driven Topological Insulator Transition in GaAs/Ge/GaAs Quantum Wells

Dong Zhang[1], Wenkai Lou[1], Maosheng Miao[2], Shou-cheng Zhang[3] and Kai Chang[1]

[1]*SKLSM, Institute of Semiconductors, Chinese Academy of Sciences, P.O. Box 912, Beijing 100083, China*

[2]*Materials Research Laboratory and Materials Department, University of California, Santa Barbara, California 93106-5050, USA and*

[3]*Department of Physics, Stanford University, Stanford, CA94305*

(Dated: July 3, 2013)

## I. 30-BAND $\boldsymbol{k} \cdot \boldsymbol{p}$ MODEL

The 30-band $\boldsymbol{k} \cdot \boldsymbol{p}$ method is known to be very efficient to describe the band structure of semiconductors in the whole Brillouin zone with reasonable accuracy. Cardona and Pollak[1] developed a 15-band (without spin) $\boldsymbol{k} \cdot \boldsymbol{p}$ model to reproduce the band structure of silicon and germanium. Richard *et al.*[2] extended it to a 30-band model after taking the spin-orbit interaction (SOI) into account.

Since the Bloch functions at $\boldsymbol{k} = 0$ form a complete set of periodic functions, it is possible to expand the cell periodic part of the wave functions at any value of $\boldsymbol{k}$ in terms of the Bloch function at $\boldsymbol{k} = 0$. Therefore, the diagonalization of the $\boldsymbol{k} \cdot \boldsymbol{p}$ Hamiltonian referred to the basis states at $\boldsymbol{k} = 0$ should yield the correct energy bands and wave functions across the entire Brillouin Zone (B.Z.) if enough basis states are taken. With the limit of empty lattice approximation, where the periodic potential $V \to 0$ while the symmetry of B.Z. (lattice periodicity) is preserved, all of these points $(2\pi/a\,(\pm 1, \pm 1, \pm))$ map the $\Gamma$ point ($\boldsymbol{k} = 0$) to equivalent centers of neighboring B.Z.'s. The large energy gap between the $2\pi/a[200]$ and the $2\pi/a[220]$ plane waves (more than $15eV$) suggests that the 15 states used correspond to free-electron states having plane waves (in units of $2\pi/a$) [000], [111], and [200] are enough to obtain the correct energy bands across the entire zone for germanium and silicon without spin-orbit interaction.[1] Introducing the spin-orbit coupling doubles the number of states to obtain the thirty-band $\boldsymbol{k} \cdot \boldsymbol{p}$ Hamiltonian.[2] In this paper, we first use the 30-band model to describe Ge/GaAs quantum well in the [111] direction. Then, starting from this 30-band model, we reduce a 4-band effective Hamiltonian to describe topological properties of Ge/GaAs Hall bar structure.[4]

The single-particle Schrödinger equation in a semiconductor bulk material is

$$H\psi = \left[\frac{\boldsymbol{p}^2}{2m_0} + V(\boldsymbol{r}) + \frac{\hbar}{4m_0^2c^2}(\nabla V \times \boldsymbol{p}) \cdot \boldsymbol{\sigma}\right]\psi = E\psi, \tag{1}$$

where $V(\boldsymbol{r})$ is a potential having the periodicity of the lattice, $m_0$ is the free electron mass, and the third term is the SOI. The solution of to Eq. (1) are Bloch function $\Psi = \exp(i\boldsymbol{k} \cdot \boldsymbol{r})\, u_{n,k}(\boldsymbol{r})$, where $u_{n,k}(\boldsymbol{r})$ has the periodicity of the crystal lattice. Eq. (1) becomes

$$\begin{aligned} H_{so}u_{n,k}(\boldsymbol{r}) &= \left[\frac{\boldsymbol{p}^2}{2m_0} + V(\boldsymbol{r}) + \frac{\hbar^2\boldsymbol{k}^2}{2m_0} + \frac{\hbar}{m_0}\boldsymbol{k} \cdot \boldsymbol{p} + \frac{\hbar}{4m_0^2c^2}(\nabla V \times \boldsymbol{p}) \cdot \boldsymbol{\sigma}\right] u_{n,k}(\boldsymbol{r}) \\ &= E_{n,k}(\boldsymbol{r})\, u_{n,k}(\boldsymbol{r}). \end{aligned} \tag{2}$$

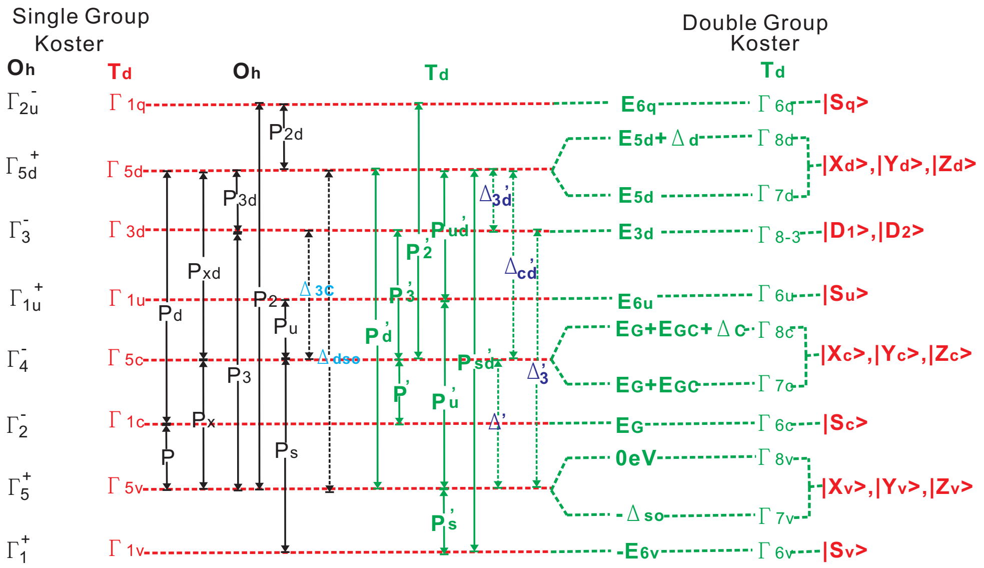


FIG. 1: The symmetry of wavefunctions use in the 30-band k.p model at $k = 0$. Left: $O_h$ and $T_d$ single group notations. Right: $T_d$ double group notation.

Fig. 1 shows schematically the basis functions at $\boldsymbol{k} = 0$ used in the 15- and 30-band models [1, 2]. The Bloch functions at $\Gamma$ point can be classified according to their irreducible presentations. For $O_h$ group semiconductors (Si and Ge), the ten $\boldsymbol{k} \cdot \boldsymbol{p}$ matrix elements of interest are: $P = (\hbar/m_0)\langle S|p_x|iX\rangle$, $P_d = (\hbar/m_0)\langle S|p_x|iX_d\rangle$, $P_X = (\hbar/m_0)\langle X_C|p_y|iZ\rangle$, $P_{Xd} = (\hbar/m_0)\langle X_C|p_y|iZ_d\rangle$, $P_3 = (\hbar/m_0)\langle D_1|p_x|iX\rangle$, $P_{3d} = (\hbar/m_0)\langle D_1|p_x|iX_d\rangle$, $P_2 = (\hbar/m_0)\langle S_2|p_x|iX\rangle$, $P_{2d} = (\hbar/m_0)\langle S_2|p_x|iX_d\rangle$, $P_s = (\hbar/m_0)\langle S_v|p_x|iX_C\rangle$, $P_U = (\hbar/m_0)\langle S_U|p_x|iX_C\rangle$. The green line represent the additional eight $k \cdot p$ matrix elements which have to be taken into account for the $T_d$ group, because of lacking of inversion symmetry. These are matrix elements: $P' = (\hbar/m_0)\langle S|p_x|iX_C\rangle$, $P_d' = (\hbar/m_0)\langle X_d|p_y|iZ\rangle$, $P_3' = (\hbar/m_0)\langle D_1|p_x|iX_C\rangle$, $P_2' = (\hbar/m_0)\langle S_2|p_x|iX_C\rangle$, $P_s' = (\hbar/m_0)\langle S_v|p_x|iX\rangle$, $P_{Sd}' = (\hbar/m_0)\langle S_v|p_x|iX_d\rangle$, $P_U' = (\hbar/m_0)\langle S_U|p_x|iX\rangle$, $P_{Ud}' = (\hbar/m_0)\langle S_U|p_x|iX_d\rangle$.

Let us now consider the effect of SOI on these states. $\Delta_{so}$, $\Delta_C$, $\Delta_d$ is the spin splitting introduced in the $\Gamma_5$ levels by the SOI. $\Delta_{dso}$, $\Delta_{Cd}'$, $\Delta'$ is the spin-orbit coupling between different $\Gamma_5$ levels. $\Delta_{3C}$, $\Delta_3'$, $\Delta_{3d}'$ are the spin-orbit coupling between $\Gamma_3$ level and $\Gamma_5$ levels. These notations are shown schematically in Fig. (1). The quantities of these parameter in our calculation are shown in Table I.

TABLE I: Matrix elements of the energies $E_{Pj}^{(\prime)} = \left(2m_0/\hbar^2\right)\left[P_j^{(\prime)}\right]^2$ defined in Fig. (1).

| Parameter | Ge(eV) | Si(eV) | GaAs(eV) | Parameter | Ge(eV) | Si(eV) | GaAs(eV) |
|---|---|---|---|---|---|---|---|
| $E_p$ | 24.60 | 19.96 | 22.37 | $E_{Pd}$ | 0.0051 | 1.193 | 0.010 |
| $E_{pX}$ | 17.65 | 14.81 | 16.79 | $E_{PXd}$ | 12.23 | 7.491 | 4.344 |
| $E_{p3}$ | 5.212 | 4.475 | 4.916 | $E_{PXd}$ | 15.76 | 9.856 | 8.888 |
| $E_{p2}$ | 2.510 | 3.933 | 6.280 | $E_{PXd}$ | 27.59 | 20.76 | 23.15 |
| $E_{pS}$ | 1.071 | 1.092 | 2.434 | $E_{PXd}$ | 17.84 | 16.36 | 19.63 |
| $E_p'$ | | | 0.0656 | $E_{Pd}',E_{P3}',E_{P2}',E_{PS}',E_{PU}',E_{PSd}',E_{PUd}' = 0$ | | | |

## II. 30-BAND MODEL FOR QUANTUM WELL ALONG ARBITRARY GROWTH DIRECTIONS

Recently, the 30-band $\boldsymbol{k}\cdot\boldsymbol{p}$ formalism which provides a description of the conduction band all over the Brillouin zone was applied to quantum wells.[3]

Next we will give the 30-band Hamiltonian for quantum wells and/or supperlattices along the arbitrary crystallographic direction,

$$\begin{aligned} \boldsymbol{r}'_{hkl} &= R\boldsymbol{r}_{001}, \\ \boldsymbol{k}'_{hkl} &= R\boldsymbol{k}_{001}, \end{aligned} \tag{3}$$

where the Euler rotation matrix is

$$R = \begin{bmatrix} \cos\varphi\cos\theta & \cos\theta\sin\varphi & -\sin\theta \\ -\sin\varphi & \cos\varphi & 0 \\ \cos\varphi\sin\theta & \sin\varphi\sin\theta & \cos\theta \end{bmatrix} \tag{4}$$

The relation between the Hamiltonians in [001] and [$hkl$] planes is

$$\cos\theta = \frac{l}{\sqrt{h^2+k^2+l^2}} \tag{5}$$

$$\cos\varphi = \frac{h}{\sqrt{h^2+k^2}} \tag{6}$$

$$\begin{cases} k'_{\alpha'} = \sum_{\alpha=x,y,z} R_{\alpha'\alpha} k_\alpha \\ k_\alpha = \sum_{\alpha'=x',y',z'} R^{-1}_{\alpha\alpha'} k'_{\alpha'} \end{cases} \tag{7}$$

$$H = \sum_{\alpha,\beta=x,y,z} k_\alpha D^{(001)}_{\alpha\beta} k_\beta + \sum_{\alpha=x,y,z} F_\alpha k^{(001)}_\alpha + C \tag{8}$$

$$H = \sum_{\alpha',\beta'=x',y',z'} k'_{\alpha'} D^{(hkl)}_{\alpha'\beta'} k'_{\beta'} + \sum_{\alpha'=x',y',z'} F^{(hkl)}_{\alpha'} k'_{\alpha'} + C \tag{9}$$

$$\begin{cases} D^{(hkl)}_{\alpha'\beta'} = \sum_{\alpha,\beta=x,y,z} R_{\alpha'\alpha} D^{(001)}_{\alpha\beta} R^{-1}_{\beta\beta'} \\ F^{(hkl)}_{\alpha'} = \sum_{\alpha=x,y,z} R_{\alpha'\alpha} F^{(001)}_\alpha \end{cases} \tag{10}$$

The wavefunctions in the barrier (B) and in the well (A) regions can be expressed as:

$$\psi_B(r) = \psi_B(\rho, z) = \sum_l e^{i\vec{k}_\rho \cdot \rho} \chi^B(z) u_{l,k_0}(r), \tag{11}$$

$$\psi_A(r) = \psi_A(\rho, z) = \sum_l e^{i\vec{k}_\rho \cdot \rho} \chi^A(z) u_{l,k_0}(r), \tag{12}$$

here $\chi^{(A,B)}(z)$ is the envelope functions in well and barrier regions, respectively.

In quantum wells, the envelope function $\chi(z)$ satisfies the following equation:

$$H_{l,m}\chi(z) = \left\{ \begin{array}{c} \left[V(z) + \frac{\hbar^2}{2m_0}\left(\boldsymbol{k}_\rho^2 - \frac{d^2}{dz^2}\right)\right] \langle u_l | u_m \rangle \\ + \frac{\hbar}{m_0} \boldsymbol{k}_\rho \cdot \langle u_l | \boldsymbol{p}_\rho | u_m \rangle + \frac{-i\hbar}{m_0} \langle u_l | p_z | u_m \rangle \frac{\partial}{\partial z} \\ + \frac{\hbar}{4m_0^2 C^2} \langle u_l | (\nabla V \times \boldsymbol{p}) \cdot \boldsymbol{\sigma} | u_m \rangle \end{array} \right\} = E\chi(z), \tag{13}$$

where $H_{l,m}$ is the matrix element of the 30-band $k \cdot p$ Hamiltonian, $p_\rho = (p_x, p_y)$. The secular equation can be diagonilzed by the plane-wave expansion method.

## III. REDUCED EFFECTIVE HAMILTONIAN

At the Γ point, the wave functions in the 30-band $\boldsymbol{k} \cdot \boldsymbol{p}$ Hamitlonian are

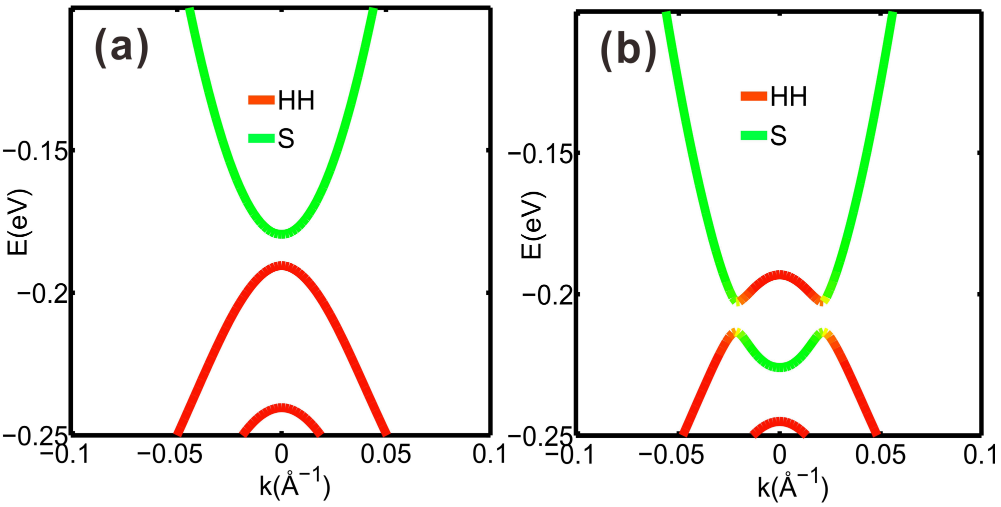


FIG. 2: (color online) Band structures of a GaAs/Ge/GaAs quantum well obtained from the thirty-band model for different thicknesses of Ge layers (a) 17.8 Å ; (b)18.3 Å . The green and red color shows the electron ($\Gamma_1$) and hole ($\Gamma_5$) components of the subbands, respectively.

$$\psi_1 = \begin{pmatrix} F_1^{(1)}(z) \\ F_2^{(1)}(z) \\ F_3^{(1)}(z) \\ F_4^{(1)}(z) \\ \vdots \\ F_{30}^{(1)}(z) \end{pmatrix} e^{ik_{//}\cdot\vec{r}}, \psi_2 = \begin{pmatrix} F_1^{(2)}(z) \\ F_2^{(2)}(z) \\ F_3^{(2)}(z) \\ F_4^{(2)}(z) \\ \vdots \\ F_{30}^{(2)}(z) \end{pmatrix} e^{ik_{//}\cdot\vec{r}}, \cdots\cdots, \psi_m = \begin{pmatrix} F_1^{(m)}(z) \\ F_2^{(m)}(z) \\ F_3^{(m)}(z) \\ F_4^{(m)}(z) \\ \vdots \\ F_{30}^{(m)}(z) \end{pmatrix} e^{ik_{//}\cdot\vec{r}}, \quad (14)$$

which can be obtained by solving the secular equation $H^{(0)}_{30\times 30}\psi_m = E_m\psi_m$.

Considering the lowest electron subband and highest heavy-hole and light-hole subbands, we obtain the effective two-dimensional Hamiltonian by averaging the $z$ component in the Hamiltonian

$$H_{eff}(\mathbf{k}_{\|}) = \langle\Psi(z)|H|\Psi(z)\rangle, \quad (15)$$

where the matrix element of the Hamiltonian is

$$
\begin{aligned}
\langle H_{eff}\rangle_{mn} &= \left\langle \psi^{(m)}\right| H_{30\times30} \left|\psi^{(n)}\right\rangle \\
&= \int \left( F_1^{*(m)}(z)\ F_2^{*(m)}(z)\ \cdots\cdots\ F_{29}^{*(m)}(z)\ F_{30}^{*(m)}(z) \right) (H)_{30\times30} \begin{pmatrix} F_1^{(n)}(z) \\ F_2^{(n)}(z) \\ \vdots \\ F_{29}^{(n)}(z) \\ F_{30}^{(n)}(z) \end{pmatrix} dz \\
&= \sum_{i,j=1}^{30} \langle F_i^{(m)}(z)\,|H_{ij}|F_j^{(n)}(z)\rangle. \qquad (16)
\end{aligned}
$$

The Hamiltonian can be divided into

$$H = H^{(0)} + H' \qquad (17)$$

$$H'\left(\mathbf{q},\hat{k}_z\right) = \alpha(\mathbf{q}) + \beta(\mathbf{q})\,\hat{k}_z + \gamma(\mathbf{q})\,\hat{k}_z^2. \qquad (18)$$

Then we have

$$
\begin{aligned}
\langle H_{eff}\rangle_{mn} = E_m\delta_{m,n} + \sum_{i,j=1}^{30} &\left\langle F_i^{(m)}(z)\right| [\alpha(\mathbf{q})]_{ij}\,|F_j^{(n)}(z)\rangle + \langle F_i^{(m)}(z)\,|\,[\beta(\mathbf{q})]_{ij}\,\hat{k}_z|F_j^{(n)}(z)\rangle \\
&+ \langle F_i^{(n)}(z)\,|\,[\gamma(\mathbf{q})]_{ij}\,\hat{k}_z^2|F_j^{(n)}(z)\rangle. \qquad (19)
\end{aligned}
$$

The contribution of the subbands other than the lowest electron and the highest hole subbands should also be considered in the reducing process. This can be done by using Löwdin perturbation theory [5], which is different from that in Ref. (4). We include the lowest 10 subbands for electron and heavy hole states respectively and divide them into the weakly coupled subsets $A$ and $B$. The set $A$ includes the lowest electron subband $|E_1\rangle$ and the highest heavy hole subbands $|HH_1\rangle$, the other subbands are included in the set $B$. The Hamiltonian is reduced into set $A$ using the Löwdin perturbation method,

$$H^{(2)}_{mm'} = \frac{1}{2}\sum_l H^{'}_{ml}H^{'}_{lm'}\left[\frac{1}{E_m - E_l} + \frac{1}{E_{m'} - E_l}\right], \qquad (20)$$

where the indices $m$ correspond to states in the set $A$, the indices $l$ correspond to states in the set $B$, and

$$H^{'}_{ml} = \langle\psi_m|\,H'\,|\psi_l\rangle\,. \qquad (21)$$

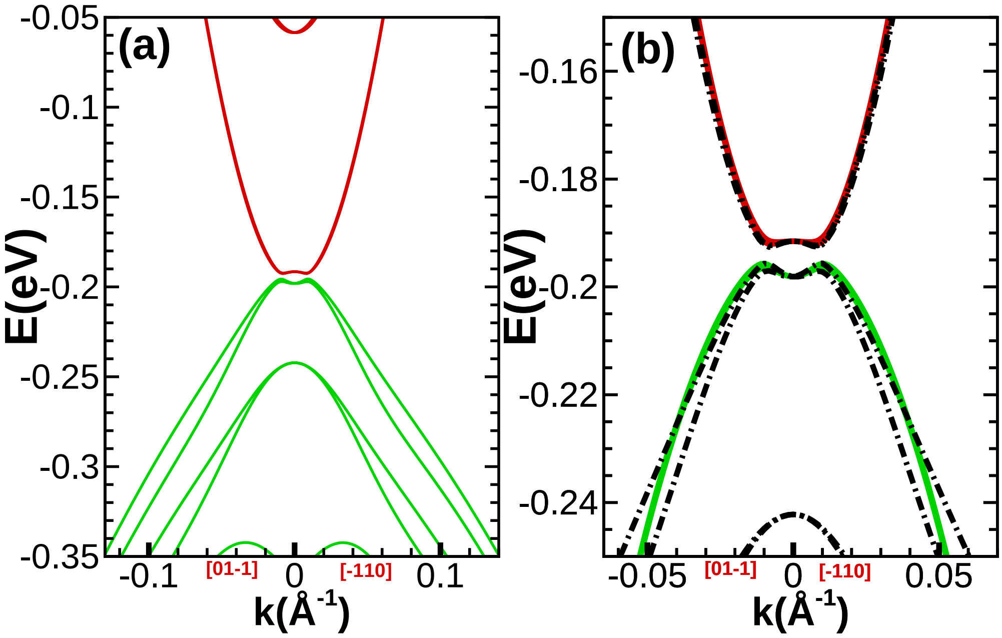


FIG. 3: (color online) Band structures of a GaAs/Ge/GaAs QW with Ge layer thickness of 18 Å obtained from the thirty-band model (the left panel and the dashed lines in the right panel) and the reduced four-band model (the solid lines in the right panel).

Finally we obtain the effective two-dimenional Hamiltonian in the basis $|E_1, \uparrow\rangle$, $|HH_1, \uparrow\rangle$, $|E_1, \downarrow\rangle$, $|HH_1, \downarrow\rangle$:

$$H^{eff}_{4\times4} = \begin{bmatrix} E_0 + E_1 k_\parallel^2 & A_1 k_+ & 0 & 0 \\ A_1^* k_- & H_0 + H_1 k_\parallel^2 & 0 & 0 \\ 0 & 0 & E_0 + E_1 k_\parallel^2 & -A_1 k_- \\ 0 & 0 & -A_1^* k_+ & H_0 + H_1 k_\parallel^2 \end{bmatrix} \tag{22}$$

where

$$E_0 = -0.19808 \ \text{eV}$$
$$E_1 = 0.43810 \ \text{eV} \cdot \text{Å}^2$$
$$H_0 = -0.19153 \ \text{eV}$$
$$H_1 = -0.20810 \ \text{eV} \cdot \text{Å}^2$$
$$A_1 = 0.028510 \ \text{eV} \cdot \text{Å}$$

In order to examine the validity of the 4-band Hamiltonian, we plot the band structure of the Ge/GaAs QW calculated by the 4-band model and compare it with the full 30-band

$\boldsymbol{k} \cdot \boldsymbol{p}$ model. The results are shown in Fig. 3. One can see clearly that the band structure obtained from the 4-band model [Fig. 3(b)] is in good agreement with that obtained from the 30-band model [Fig. 3(a)].


[1] M. Cardona, N. E. Christensen, and G. Fasol, Phys. Rev. B **38**, 1806 (1988).

[2] S. Richard, F. Aniel, and G. Fishman, Phys. Rev. B **70**, 235204 (2004).

[3] M. El Kurdi, S. Sauvage, G. Fishman, and P. Boucaud, Phys. Rev. B **73**, 195327 (2006).

[4] B. A. Bernevig, T. L. Hughes, and S. C. Zhang, Science **314**, 1757 (2006).

[5] P. O. Löwdin. J. Chem. Phys. **19**, 1396 (1951).
